# Supplementary material for: On-the-Fly Power-Aware Rendering
Source: arXiv:1807.11760 ancillary file (2018-07-31)
Supplement: Supplementary file 1 [file supplementary.pdf]

Eurographics Symposium on Rendering 2018
T. Hachisuka and W. Jakob
(Guest Editors)

*Volume 37 (2018), Number 4*

# On-the-Fly Power-Aware Rendering Supplementary Material

Yunjin Zhang[1*] Marta Ortin[2*] Victor Arellano[2] Rui Wang[1] Diego Gutierrez[2] Hujun Bao[1]

[1] State Key Lab of CAD&CG, Zhejiang University [2] Universidad de Zaragoza, I3A
*Joint first authors

This document includes additional results demonstrating the accuracy of our power prediction model in all the demo scenes, and shows the effect of using different power budgets.

## 1. Accuracy of our real-time power prediction model

Figure 1 shows the accuracy of our power prediction model in all our demo scenes for several rendering configurations, and includes the prediction obtained with the model proposed by Vatjus-Anttila et al. [VAKH13] for comparison. Figures 2 and 3 depict additional results to show the accuracy of our power prediction model.

## 2. Effect of the power budget

The trade-off between power consumption and image quality depends on the characteristics of each scene, some of them being able to save more power with less image quality degradation. The results obtained with our framework span from no power savings and perfect image quality (100% power budget) to maximum power savings and worst image quality (0% power budget). Figure 4 shows the impact of power budgets 50% and 60% on the resulting power and quality error for the *Sponza* scene. With 60% power budget, we are able to obtain power savings with minimal quality degradation. Reducing the power budget to 50% allows us to save more power, but produces higher image error. In a real application, this power budget can be adjusted in real time based on the requirements of the user.

## References

[VAKH13] Vatjus-Anttila J. M., Koskela T., Hickey S.: Power consumption model of a mobile GPU based on rendering complexity. In *2013 Seventh International Conference on Next Generation Mobile Apps, Services and Technologies* (Sept 2013), pp. 210–215. doi:10.1109/NGMAST.2013.45. 1, 2

© 2018 The Author(s)
Computer Graphics Forum © 2018 The Eurographics Association and John Wiley & Sons Ltd. Published by John Wiley & Sons Ltd.

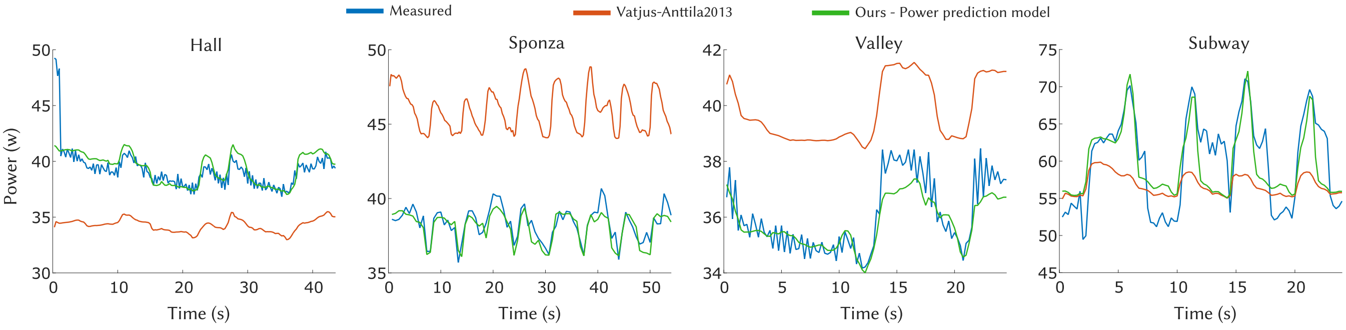


(a) Rendering configuration $\mathbf{s} = (l_0, l_0, l_0, l_0, l_0, l_0)$

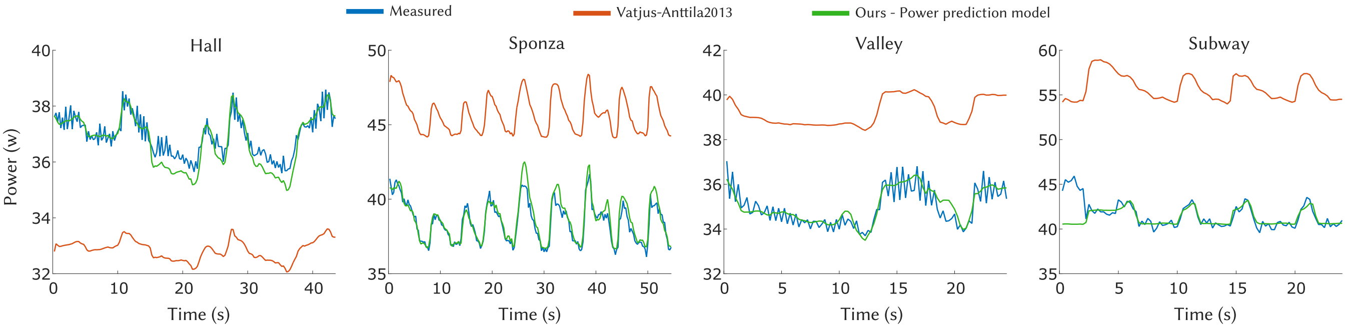


(b) Rendering configuration $\mathbf{s} = (l_1, l_1, l_1, l_1, l_1, l_1)$

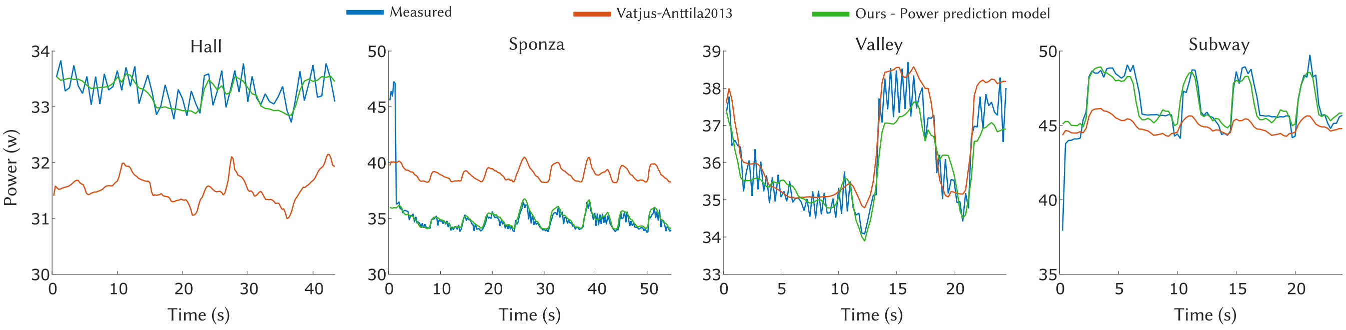


(c) Rendering configuration $\mathbf{s} = (l_2, l_2, l_2, l_2, l_2, l_2)$

**Figure 1:** *Power consumption of our four demo scenes (Hall, Sponza, Valley, and Subway) with different rendering configurations. We show ground truth measured data, predicted power with our real-time fitting, and the prediction using the model proposed by Vatjus-Anttila et al. [VAKH13]. Note that predictions with Vatjus-Anttila et al.'s model either present an offset with respect to ground truth data, or report power within the same range of values but fail to capture the peaks and valleys.*

© 2018 The Author(s)
Computer Graphics Forum © 2018 The Eurographics Association and John Wiley & Sons Ltd.

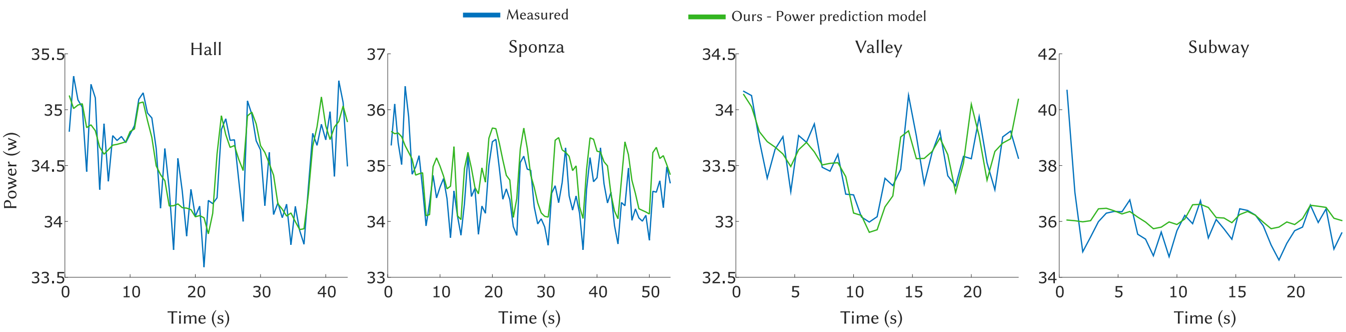


(a) Rendering configuration $\mathbf{s} = (l_0, l_2, l_1, l_1, l_1, l_1)$

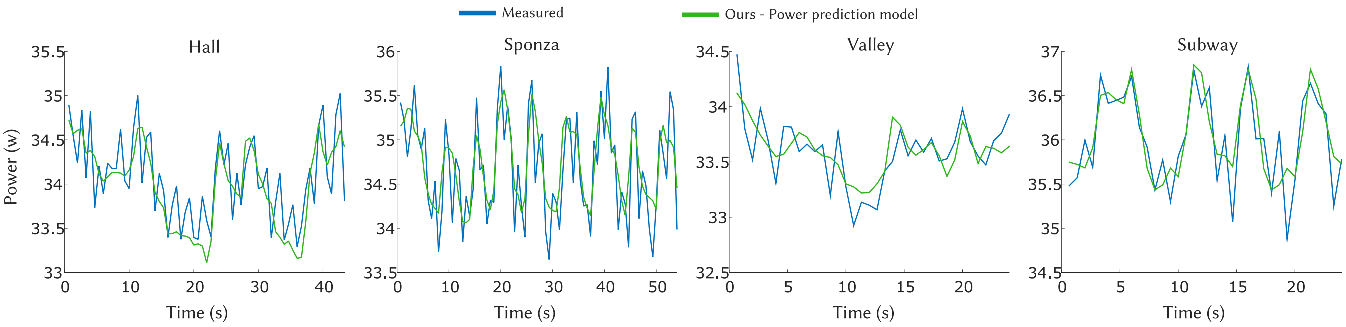


(b) Rendering configuration $\mathbf{s} = (l_0, l_2, l_1, l_1, l_2, l_2)$

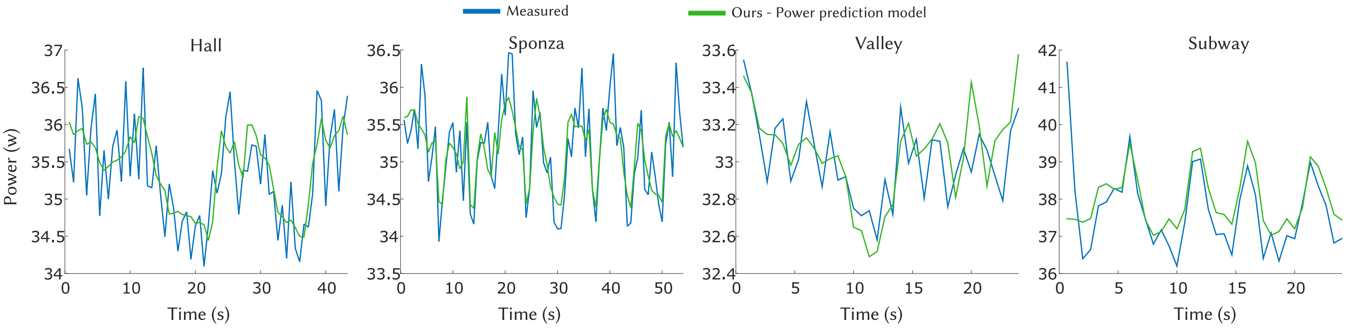


(c) Rendering configuration $\mathbf{s} = (l_1, l_1, l_2, l_0, l_0, l_1)$

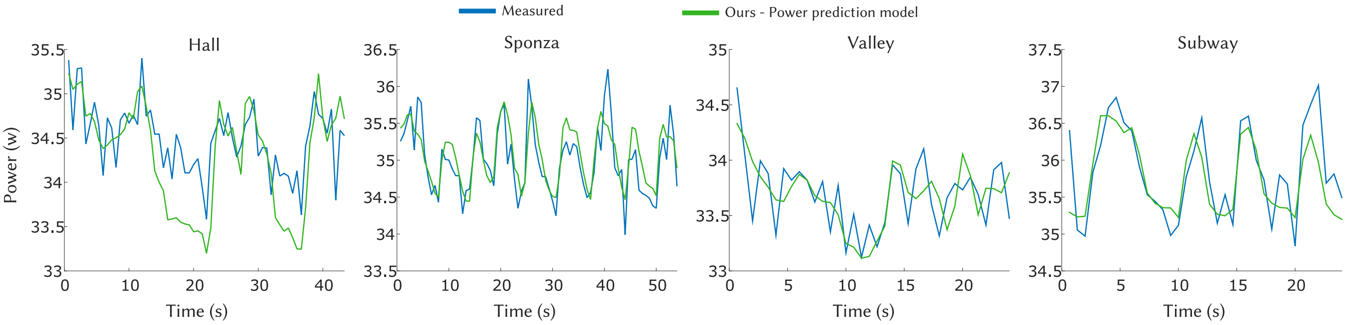


(d) Rendering configuration $\mathbf{s} = (l_1, l_2, l_0, l_0, l_2, l_0)$

**Figure 2:** *Power consumption of our four demo scenes (Hall, Sponza, Valley, and Subway) demo scenes, for different rendering configurations. We show ground truth measured data and predicted power with our real-time fitting.*

© 2018 The Author(s)
Computer Graphics Forum © 2018 The Eurographics Association and John Wiley & Sons Ltd.

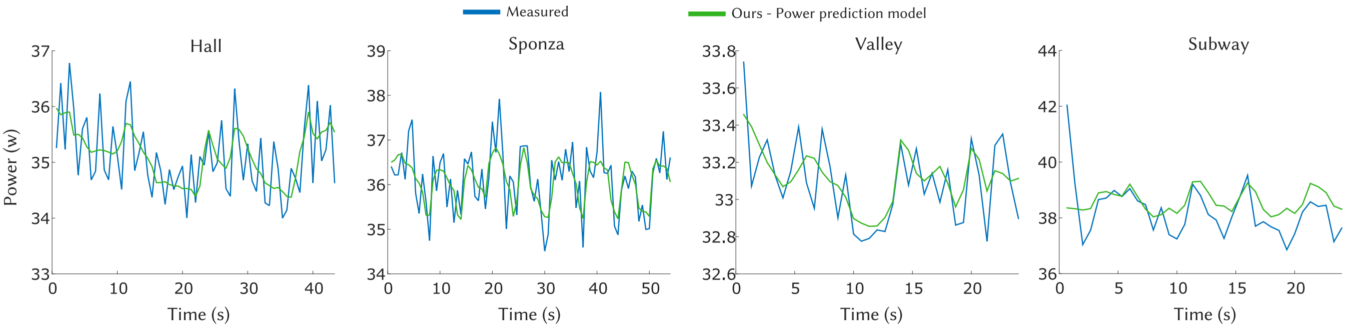


(a) Rendering configuration $\mathbf{s} = (l_2, l_0, l_0, l_2, l_1, l_0)$

**Figure 3:** *Power consumption of our four demo scenes (Hall, Sponza, Valley, and Subway) demo scenes, for different rendering configurations. We show ground truth measured data and predicted power with our real-time fitting.*

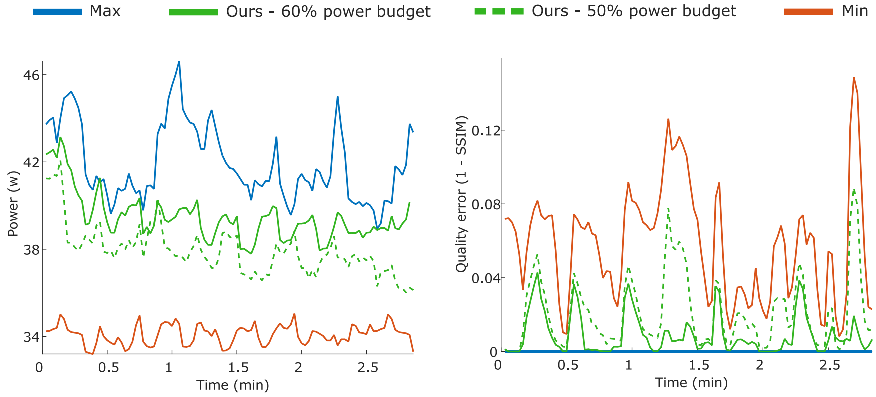


**Figure 4:** *Comparison of the minimum and maximum rendering configurations against two of our results: with power budgets of 60% and 50%. Graphs correspond to the Sponza scene executed on a desktop PC.*

© 2018 The Author(s)
Computer Graphics Forum © 2018 The Eurographics Association and John Wiley & Sons Ltd.
